# Supplementary material for: NEREL-BIO: A Dataset of Biomedical Abstracts Annotated with Nested Named Entities
Source: arXiv:2210.11913 source file (2022-10-21)
Supplement: Supplementary file 1 [file supplement.tex]

% \documentclass[b4paper]{bioinfo}
% \copyrightyear{2020} \pubyear{2020}

% \usepackage[utf8]{inputenc}
% \usepackage[T1]{fontenc}

% \usepackage[english]{babel}

% \usepackage{fontspec}
% \setmainfont[Ligatures=TeX]{CMU Serif}
% \usepackage{polyglossia}
% \setdefaultlanguage{english}
% \setotherlanguage{russian}

% \setcounter{table}{0}
% \renewcommand{\thetable}{S\arabic{table}}
% \renewcommand{\thefigure}{S\arabic{figure}}

% \begin{document}

% \subtitle{Supplementary}

% \title{The Russian Drug Reaction Corpus and Neural Models for Drug Reactions and Effectiveness Detection in User Reviews}

% \author[]{Elena Tutubalina, Ilseyar Alimova, Zulfat Miftahutdinov, Andrey Sakhovskiy, Valentin Malykh, Sergey Nikolenko}

% \abstract{
% The Russian Drug Reaction Corpus (\textsc{RuDReC}) is a new partially annotated corpus of consumer reviews in Russian about pharmaceutical products for the detection of health-related named entities and the effectiveness of pharmaceutical products.
% The corpus itself consists of two parts, the raw one and the labelled one. The raw part includes 1.4 million health-related user-generated texts collected from various Internet sources, including social media.
% The labelled part contains 500 consumer reviews about drug therapy with drug- and disease-related information. Labels for sentences include health-related issues or their absence. The sentences with one are additionally labelled at the expression level for identification of fine-grained subtypes such as drug classes and drug forms, drug indications, and drug reactions. %which is significantly larger than any previous health-related corpus. 
% Further, we present a baseline model for named entity recognition (NER) and multi-label sentence classification tasks on this corpus. The macro F1 score of 74.85\% in the NER task was achieved by our RuDR-BERT model. For the sentence classification task, our model achieves the macro F1 score of 68.82\% gaining 7.47\% over the score of BERT model trained on Russian data.\\
% \textbf{Availability:} We make the RuDReC corpus and pretrained weights of domain-specific BERT models freely available at \url{https://github.com/cimm-kzn/RuDReC}
% }

% \maketitle

% \section{Supplementary}

% Supplementary Table S1 presents statistics on existing relevant corpora: 
% \begin{itemize}
% \item Alimova, I., Tutubalina, E., Alferova, J., and Gafiyatullina, G. (2017). A machine learning approach to classification of drug reviews in russian. In
% 2017 Ivannikov ISPRAS Open Conference (ISPRAS), pages 64–69. IEEE.
% \item Alvaro, N., Miyao, Y., and Collier, N. (2017). Twimed: Twitter and pubmed comparable corpus of drugs, diseases, symptoms, and their relations. JMIR
% public health and surveillance, 3(2).
% \item Moreno, I., Boldrini, E., Moreda, P., and Romá-Ferri, M. T. (2017). Drugsemantics: a corpus for named entity recognition in spanish summaries of
% product characteristics. Journal of biomedical informatics, 72, 8–22.
% \item Karimi, S., Metke-Jimenez, A., Kemp, M., and Wang, C. (2015). Cadec: A corpus of adverse drug event annotations. Journal of biomedical informatics, 55, 73–81.
% \item Shelmanov, A., Smirnov, I., and Vishneva, E. (2015). Information extraction from clinical texts in russian. volume 1, pages 560–572.
% \item Zolnoori, M., Fung, K. W., Patrick, T. B., Fontelo, P., Kharrazi, H., Faiola, A., Wu, Y. S. S., Eldredge, C. E., Luo, J., Conway, M., et al. (2019). A systematic approach for developing a corpus of patient reported adverse drug events: A case study for ssri and snri medications. Journal of biomedical informatics, 90, 103091.
% \end{itemize}

% \begin{table*}[!h]
% \processtable{Basic statistics of existing drug-related text corpora.\label{tab:corpora}} {\begin{tabular}{@{}p{3.4cm}p{2.cm}p{1.7cm}p{1.7cm}p{5.cm}@{}}
% \toprule 
% \textbf{Corpus} & \textbf{Text type} & \textbf{No. of texts} & \textbf{No. of entities} & \textbf{Annotations} \\ 
% %  & & \textbf{texts} & \textbf{entities} &  \\ 
% \midrule
% \multicolumn{5}{c}{\textbf{English language corpora}} \\ \hline
% CADEC, Karimi et al.(2015)  & User reviews & 1253 & 9111 & ADR, Disease, Symptom, Finding, Drug\\ %\hline
% PsyTAR, Zolnoori et  al.(2019) & User reviews  & 887 & 7414 & ADR, Withdrawal symptom, symptoms, drug indication (DI) \\ %\hline
% TwiMed, Alvaro et al.(2017 & \raggedright Sentences from abstracts, tweets & 2000 & 3144 &  Drug, Symptom, Diseases\\ %\hline
% %SMM4H 2017~\cite{10.1093/jamia/ocy114} & tweets & 25678 & N/A & 25678 tweets annotated to indicate the presence or absence of ADRs \\
% \hline
% \multicolumn{5}{c}{\textbf{Spanish language corpora}} \\ \hline
% Drug Semantics, Moreno et al.(2017) & \raggedright Summaries of Product Characteristics & 5 & 2241 & Disease, Drug, Unit of Measurement, Excipient, Chemical Composition, Pharmaceutical Form, Route, Medicament Food and Therapeutic Action \\ %\hline
% \hline
% \multicolumn{5}{c}{\textbf{Russian language corpora}} \\ \hline
% Shelmanov et al., 2015 & Clinical notes  & 112 & 7600 & Disease, Symptom, Drug, Treatment, Body location, Severity, Course \\ %\hline
% Alimova et al., 2017 & Reviews' sentences & 370 & N/A & Sentences from reviews annotated with the presence of Indication, Beneficial effect, ADR, Other \\ %\hline
% SMM4H 2020 Task & Tweets & 9515 & N/A & Tweets annotated with presence of ADRs \\ 
% \textsc{RuDReC} (ours) & User reviews & 500 & 4566 & DI, ADR, Finding, Drug name, Drug class, Drug form \\
% \botrule
% \end{tabular}}{}
% \end{table*}
% % \hline
% % \end{tabular}
% % \end{center}
% % \end{table*}

% Supplementary Figure \ref{fig:pharm_group} and \ref{fig:pharm_rating} present statistics on therapeutic groups and ratings in our corpus, respectively. 
% Every user fills out this information as well as 5-star ratings when writing a review. The majority of the reviews (60\%) are describing the antiviral drugs, which are of the most common ones used in everyday life. 
% The second by number group is sedatives and antidepressants (27\%), which are on the raise in recent years. Another interesting feature is that the prevalence of the highest rating (5) is not overpowering the other ratings, which are more or less uniformly distributed. This is a common feature that the intermediate rating is mostly skipped in many domains, but the collected data is showing unusual uniformity. 

% % \begin{figure*}
% %   \begin{minipage}{0.50\textwidth}
% %   \centering
% %      \includegraphics[width=0.8\linewidth]{images/coling001.pdf}
% %   \end{minipage}
% %   \begin{minipage}{0.50\textwidth}
% %      \centering
% %      \includegraphics[width=0.8\linewidth]{images/coling002.pdf}
% %   \end{minipage}
% % \caption{Statistics on therapeutic groups and ratings in the annotated corpus (filled by reviews' authors).}\label{fig:statistics}  
% % \end{figure*}

% \begin{figure}[!th]
% \centerline{\includegraphics[width=0.6\linewidth]{images/coling001.pdf}}
% \caption{Statistics on therapeutic groups in the annotated corpus (filled by reviews' authors).}\label{fig:pharm_group}
% \end{figure}

% \begin{figure}[!th]
% \centerline{\includegraphics[width=0.6\linewidth]{images/coling002.pdf}}
% \caption{Statistics on ratings in the annotated corpus (filled by reviews' authors).}\label{fig:pharm_rating}
% \end{figure}

% The annotated corpus consists of 500 reviews about drugs from these four groups. Reviews were selected randomly for annotation. The examples of annotated entities for each group are presented in Supplementary Table S2. 


% \begin{table*}[!h]
% \processtable{Examples of annotated entities for four therapeutic groups} {\begin{tabular}{@{}p{1cm}p{14.5cm}@{}}
% \toprule
% \textbf{Entity} & \textbf{Examples of entities} \\
% \midrule
% \multicolumn{2}{c}{Sedatives} \\
% \hline
% DI & \foreignlanguage{russian}{бессонница (insomnia), раздражительность (irritability), стресс (stress), усталость (fatigue), чувство тревоги (anxiety)}\\
% ADR & \foreignlanguage{russian}{сонливость (drowsiness), слабость (weakness), раздражительность (irritability), апатия (apathy), головная боль (headache)}\\
% \hline
% \multicolumn{2}{c}{Immunomodulators} \\
% \hline
% DI & \foreignlanguage{russian}{ОРВИ (VRI), простуда (cold), насморк (runny nose), температура (temperature), кашель (cough)} \\
% ADR & \foreignlanguage{russian}{диарея (diarrhea), аллергия (allergy), температура (temperature), слабость (weakness), боли в мышцах (muscle pain)}\\
% \hline
% \multicolumn{2}{c}{Nootropic} \\
% \hline
% DI & \foreignlanguage{russian}{не разговаривает (not talking), задержка речевого развития (delayed speech development), отсутствие речи (lack of speech), плохо держал головку (could not hold the head), кисты в мозгу (cysts in the brain)} \\
% ADR & \foreignlanguage{russian}{бессонница (insomnia), рвота (vomiting), в стуле появилась обильная слизь (profuse mucus appeared in the stool), головная боль (headache), не спал толком (did not sleep well)} \\
% \hline
% \multicolumn{2}{c}{Antiviral} \\
% \hline
% DI & \foreignlanguage{russian}{простуда (cold), ОРВИ (VRI), грипп (flu), насморк (running nose), температура (temperature)}\\
% ADR & \foreignlanguage{russian}{аллергия (allergy), диарея (diarrhea), сыпь (rash), слабость (weakness), головная боль (headache)}\\
% \botrule
% \end{tabular}}{}
% \end{table*}





% % \begin{figure}[h]
% % \centerline{\includegraphics[width=0.6\linewidth]{images/coling001.pdf}}
% % \caption{Statistics on therapeutic groups in the annotated corpus (filled by reviews' authors).}\label{fig:pharm_group}
% % \end{figure}

% % \begin{figure}[h]
% % \centerline{\includegraphics[width=0.6\linewidth]{images/coling002.pdf}}
% % \caption{Statistics on ratings in the annotated corpus (filled by reviews' authors).}\label{fig:pharm_rating}
% % \end{figure}


% % \begin{thebibliography}
% % \newpage

% % \bibitem[Alimova {\em et~al.}(2017)Alimova, Tutubalina, Alferova, and
% %   Gafiyatullina]{alimova2017machine}
% % Alimova, I., Tutubalina, E., Alferova, J., and Gafiyatullina, G. (2017).
% % \newblock A machine learning approach to classification of drug reviews in
% %   russian.
% % \newblock In {\em 2017 Ivannikov ISPRAS Open Conference (ISPRAS)\/}, pages
% %   64--69. IEEE.

% % \bibitem[Alvaro {\em et~al.}(2017)Alvaro, Miyao, and Collier]{alvaro2017twimed}
% % Alvaro, N., Miyao, Y., and Collier, N. (2017).
% % \newblock Twimed: Twitter and pubmed comparable corpus of drugs, diseases,
% %   symptoms, and their relations.
% % \newblock {\em JMIR public health and surveillance\/}, {\bf 3}(2).

% % \bibitem[Moreno {\em et~al.}(2017)Moreno, Boldrini, Moreda, and
% %   Rom{\'a}-Ferri]{moreno2017drugsemantics}
% % Moreno, I., Boldrini, E., Moreda, P., and Rom{\'a}-Ferri, M.~T. (2017).
% % \newblock Drugsemantics: a corpus for named entity recognition in spanish
% %   summaries of product characteristics.
% % \newblock {\em Journal of biomedical informatics\/}, {\bf 72}, 8--22.

% % \bibitem[Karimi {\em et~al.}(2015)Karimi, Metke-Jimenez, Kemp, and
% %   Wang]{karimi2015cadec}
% % Karimi, S., Metke-Jimenez, A., Kemp, M., and Wang, C. (2015).
% % \newblock Cadec: A corpus of adverse drug event annotations.
% % \newblock {\em Journal of biomedical informatics\/}, {\bf 55}, 73--81.

% % \bibitem[Shelmanov {\em et~al.}(2015)Shelmanov, Smirnov, and
% %   Vishneva]{Shelmanov2015560}
% % Shelmanov, A., Smirnov, I., and Vishneva, E. (2015).
% % \newblock Information extraction from clinical texts in russian.
% % \newblock volume~1, pages 560--572.

% % \bibitem[Zolnoori {\em et~al.}(2019)Zolnoori, Fung, Patrick, Fontelo, Kharrazi,
% %   Faiola, Wu, Eldredge, Luo, Conway, {\em et~al.}]{zolnoori2019systematic}
% % Zolnoori, M., Fung, K.~W., Patrick, T.~B., Fontelo, P., Kharrazi, H., Faiola,
% %   A., Wu, Y. S.~S., Eldredge, C.~E., Luo, J., Conway, M., {\em et~al.} (2019).
% % \newblock A systematic approach for developing a corpus of patient reported
% %   adverse drug events: A case study for ssri and snri medications.
% % \newblock {\em Journal of biomedical informatics\/}, {\bf 90}, 103091.

% % \end{thebibliography}

% \end{document}
